# Supplementary material for: Intersecting Liminality: Acquiring a Smartphone as a Blind or Low Vision Older Adult
Source: arXiv:2409.03086 source file (2024-09-04)
Supplement: Supplementary file 1 [file appendix.tex]

\appendix
\section{Appendix}

% Please add the following required packages to your document preamble:
% \usepackage{graphicx}
% \usepackage[table,xcdraw]{xcolor}
% Beamer presentation requires \usepackage{colortbl} instead of \usepackage[table,xcdraw]{xcolor}
\begin{table*}[ht]
%\resizebox{\textwidth}{!}{%
\begin{tabular}{p{0.05\linewidth} 
               p{0.9\linewidth}}
               \toprule
\textbf{ID} & \textbf{Smartphone Experience (Summary)}                                                                                                                  \\
\midrule
\rowcolor[HTML]{F3F3F3} 
P1          & Android, iPhone 8 Plus \& 12 Pro Max                                                                                                                      \\
P2          & iPhone user $\approx$ 13 years, since iPhone 5. Using BlindShell for less than 1 year                                                                     \\
\rowcolor[HTML]{F3F3F3} 
P3          & iPhone SE over 1 year                                                                                                                                     \\
P4          & iPhone SE 1st and 2nd generation                                                                                                                          \\
\rowcolor[HTML]{F3F3F3} 
P5          & has used Blackberry, iPhone 4 \& 6, BlindShell. Before losing vision, P5 described using Blackberry and Android phones                                    \\
P6 &
  iPhone user $\approx$ 7 years. Used iPhones 6 \& 7 before upgrading to iPhone SE in 2023. Previously used National Braille Press smart B2G device which ran Android. Mainly use the iPhone for phone calls while not home, audio books, music, podcasts, audio described movies, and radio. \\
\rowcolor[HTML]{F3F3F3} 
P7          & uses all the time. had to learn new things with the smartphone. Has had his current smartphone for 1.5 years                                              \\
P8          & iPhone user $\approx$ 6 years, since 2017. Had a flip phone. Had an iPhone 5, 7, 8, then 12.                                                              \\
\rowcolor[HTML]{F3F3F3} 
P9          & Used an iPhone since 2011. I am a high-end user, meaning that I do a whole lot more with the iPhone than simply receiving and making phone calls.         \\
P10         & 2021 iPhone was first smartphone. uses iPhone everyday for making/receiving calls, receives messages, email, contact management, etc.                     \\
\rowcolor[HTML]{F3F3F3} 
P11         & iPhone user $\approx$ 5 to 7 years. First cell phone in year 2000. Got BlindShell after iPhone. uses smartphone when needed                               \\
P12         & Used smartphones on a daily basis since their commercial rollout, primarily for emails, texts and internet access for both professional and personal use. \\
\rowcolor[HTML]{F3F3F3} 
P13         & iPhone user $\approx$ 6 years, 4 with vision loss. used a flip phone for a long time before smartphone. Computer user of 55 years.                        \\
P14         & very dependent on iPhone and iPad. Full-time use every day learning all technological options to compensate for low vision.                               \\
\rowcolor[HTML]{F3F3F3} 
P15 &
  iPhone user $\approx$ 10 years, 3 with sight loss as a blind person. uses VoiceOver occasionally mainly to search web, make phone calls, calendar appointments. uses navigation apps for going around neighborhood and going places. \\
P16         & Use it every day to call and text. Alarms and reminders                                                                                                   \\
\rowcolor[HTML]{F3F3F3} 
P17         & iPhone user $\approx$ 3 years. Uses it all day long. Had cell phones before                                                                               \\
P18         & iPhone user $\approx$ 12 years, and before had Nokia smartphones until about 2003. pretty good at them                                                    \\
\rowcolor[HTML]{F3F3F3} 
P19         & Smartphone user for over 10 years, use them every day as a part of daily life.                                                                            \\
P20 &
  Android user $\approx$ 6 years. Before, used Simbian and Windows phones. Uses Android phone everyday. Tasks such as Bing messaging, email, directions, reading package labels, and using internet for search. \\
\rowcolor[HTML]{F3F3F3} 
P21 &
  Android user $\approx$ 10 years. Came with Android Jellybean OS. Tasks such as communication, news, notes, research, calls, and much more. Now has one with him all the time. \\
P22 &
  Has been using Android devices from the start. His first smartphone was the ADP1, the original Android device for developers. First Android phone with cell service was the Samsung Galaxy S3. Tasks such as daily research/reading of technical articles and news, search, email, messages, Google assistant extensively and some routines, radio, weather, etc. \\
  \bottomrule
\end{tabular}%
%}
\caption{Summary of Self-Reported Smartphone Experience as Described by Participants}
\label{tab:summary_exp_table}
\end{table*}
